# Supplementary material for: Topographical coloured plasmonic coins
Source: arXiv:1609.02874 source file (2016-09-09)
Supplement: Supplementary file 1 [file supplementary.pdf]

# Supplementary materials for:
Topographical coloured plasmonic coins

J-M Guay[1,2,4,*], A. Calà Lesina[1,2], G. Côté[1,2,4], M. Charron[1], L. Ramunno[1,2], P. Berini[1,2,3], and A. Weck[1,2,4]

[1]Department of Physics, University of Ottawa, ON, K1N 6N5, Canada
[2]Centre for Research in Photonics, University of Ottawa, ON, K1N 6N5, Canada
[3]School of Electrical Engineering and Computer Science, University of Ottawa, ON, K1N 6N5, Canada
[4]Department of Mechanical Engineering, University of Ottawa, ON, K1N 6N5, Canada
[*]email: jguay036@uottawa.ca

August 25, 2016

## Figure S. 1 and S. 2

The particle density ejected from the ablation of a single line was observed to differ away from the center of the groove, Figure S. 1 (c,d). The different particle density can be seen by the color gradient next to be ablated line, Figure S. 1 (a). From this information the proper spacing between subsequent lines can determined in order to tune to the desired colour. In the case of Figure S. 1 (a,b), a very slow speed was used in order to compensate for the lack of subsequent lines and in consequence produced a groove. However, for closely spaced lines no acute denivelation is observed, Figure S. 2 (a,b), and a somewhat leveled surface is formed in the colouring process. In addition due to the low electron-phonon coupling of silver [1], no distinctive LIPSS formed in the center of the irradiated line, however, LIPSS can be seen on the side of the irradiated line, Figure S. 1 (b). These LIPSS are destroyed in the coloring process with laser line spacing below the spot size and no LIPSS structures can be seen, Figure S. 2 (a,b). For line spacing large enough (i.e yellow colors) were no appreciable line overlap occurs some angle-dependence on the colors can be observed and only for certain laser parameters.

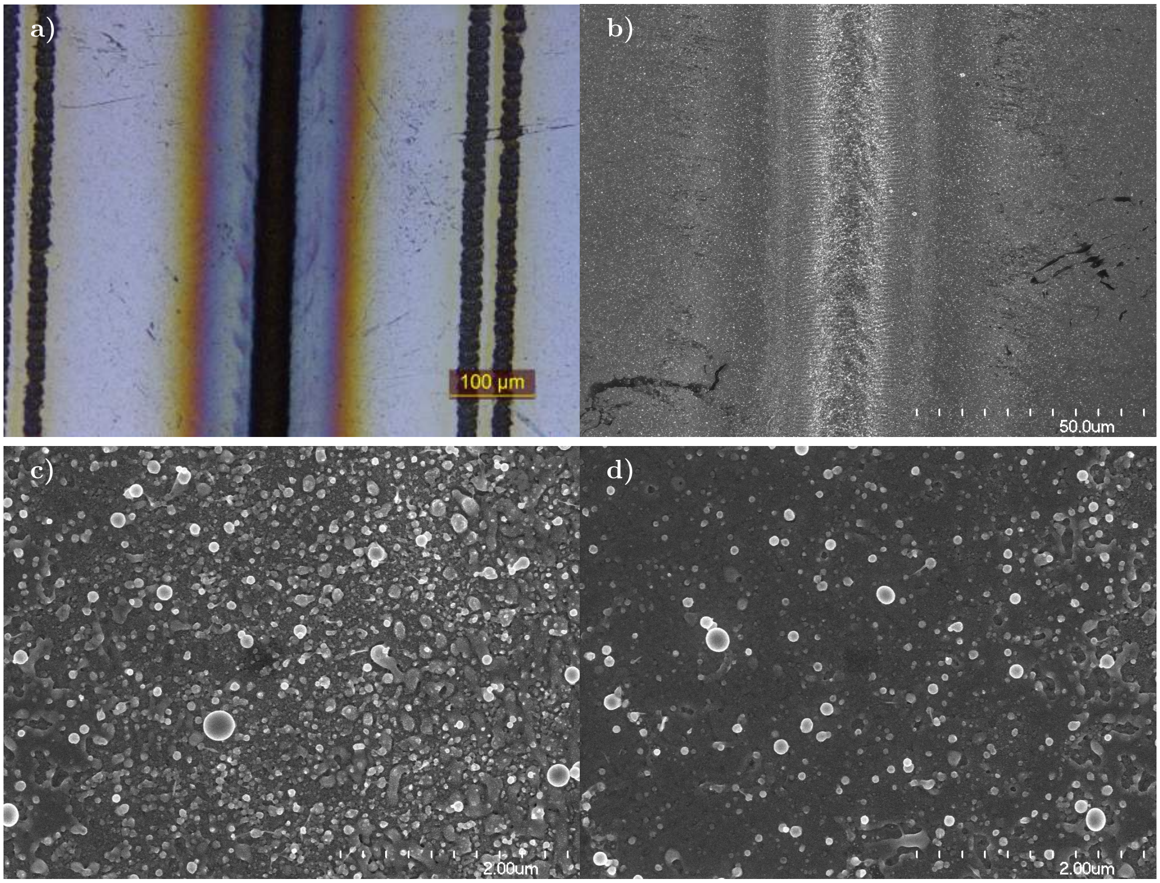


Figure S. 1: (a) Photograph taken under 50x magnification of a laser ablated line on silver. (b) SEM magnification of laser ablated line on the surface of silver and (b,c) are SEM pictures of the particles deposited next to the ablated line with (c) closer to the lasered line and (d) moving away from the center of the grove.

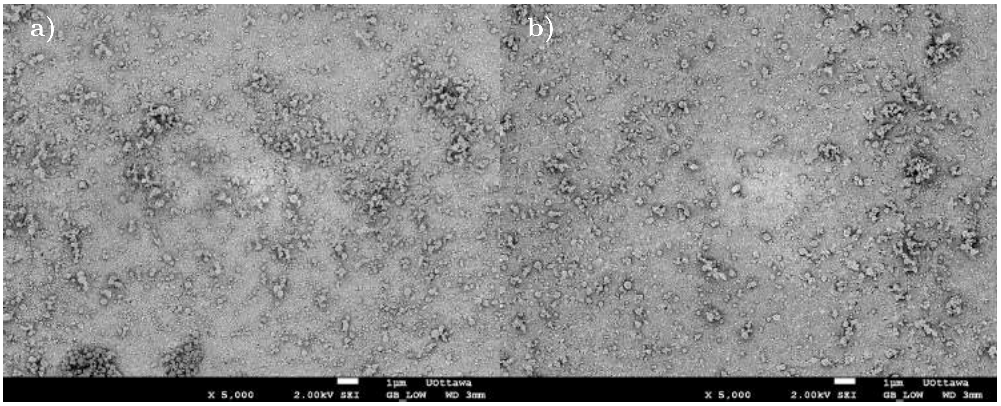


Figure S. 2: Low Magnification SEM images of coloured silver surfaces using 11 mm/s at 1.12 $J/cm^2$ with a line spacing of (a) 10 $\mu$m and (b) 13 $\mu$m.

## Figure S. 3

Surface analysis of coloured regions reveal that the number density of small particles, produced using different laser parameters, follows its own universal trend, S. 3 (a), similar to that of Fig. 1(d), whereas the number density of the medium particles does not S. 3 (b). This observation suggests that the small particles play a major role in the colours perceived, even though they have not been considered in previous works. The mean radius of small and medium nanoparticles was found to remain approximately constant as a function of line spacing, as observed in S. 3 (c,d) (determined from the analysis of 3 SEM images per line spacing, i.e., colour). However, the mean inter-particle (wall-to-wall) distance changes with line spacing, so the colours are believed to be caused by near-field interactions between nanoparticles in close proximity [2–5], particularly the associated surface plasmon resonance frequency [5].

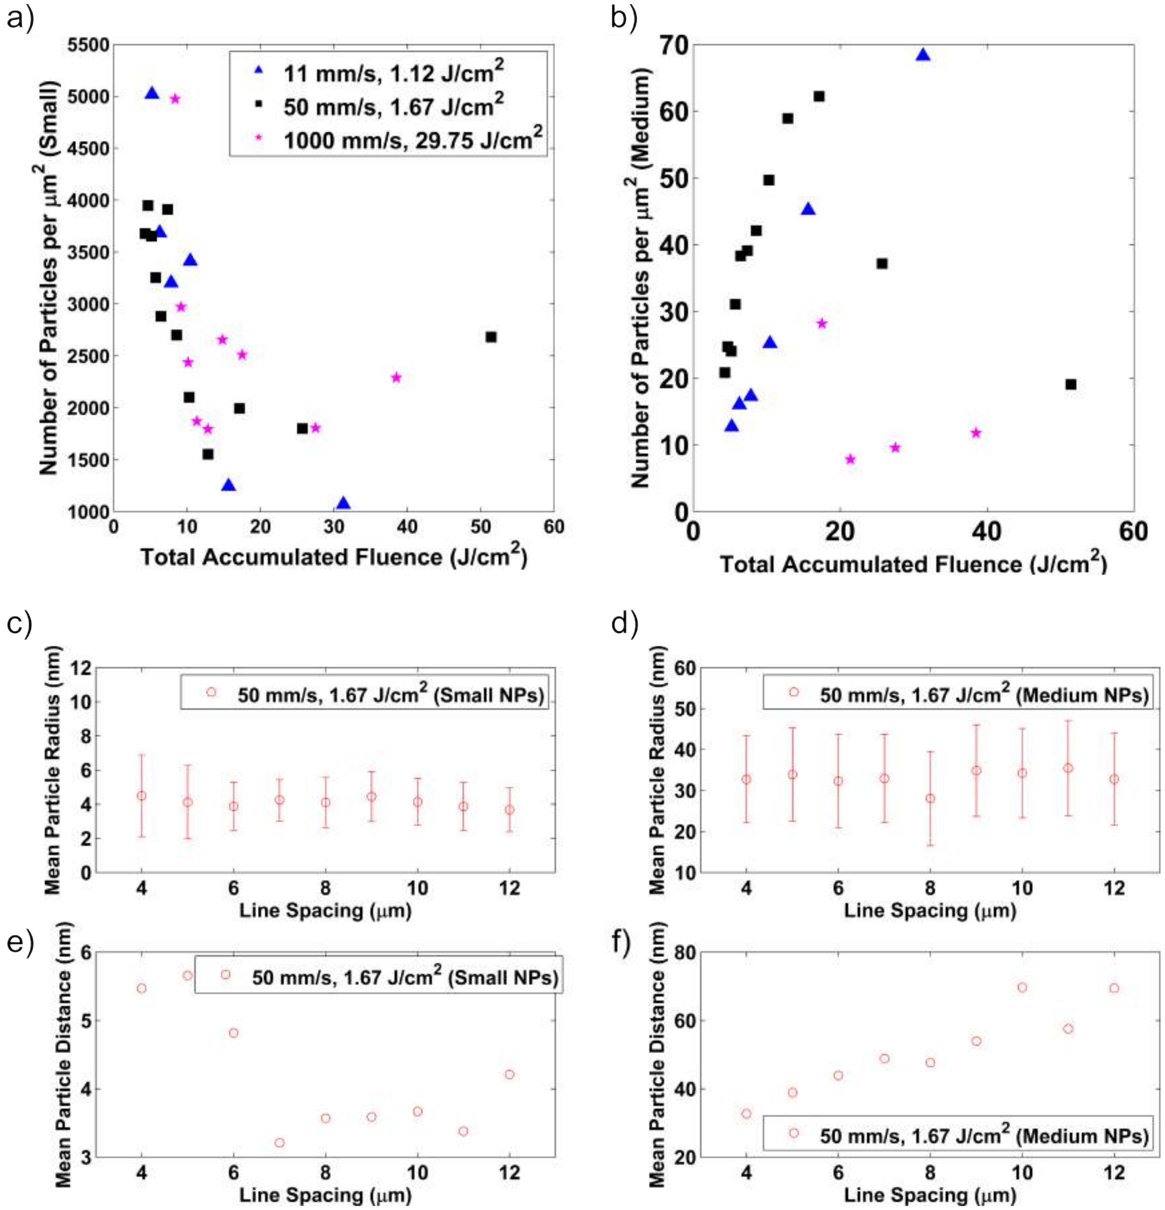


Figure S. 3: Number of particles per $\mu m^2$ versus total accumulated fluence for (a) small nanoparticles and (b) medium nanoparticles for a fluence $\phi$ = 1.12 J/cm$^2$ at laser marking speed $v$ = 11 mm/s, $\phi$ = 1.67 J/cm$^2$ at $v$ = 50 mm/s, and $\phi$ = 29.75 J/cm$^2$ at $v$ = 1000 mm/s. Mean particle radius versus line spacing for (c) small NPs and (d) medium-large NPs for $\phi$ = 1.67 J/cm$^2$ at $v$ = 50 mm/s. Mean inter-particle distance (wall-to-wall) versus line spacing for (e) small NPs and (f) medium-large NPs for $\phi$ = 1.67 J/cm$^2$ at $v$ = 50 mm/s.

## Figure S. 4

Figures S. 4 (a-c) show histograms of the number of particles on the surface over an area of 1 $\mu m^2$ versus particle radius for line spacings $L_s$ = 5, 10 and 30 $\mu$m, respectively. Two discernible bumps (bimodal distribution) are noted in the histograms, corresponding to the small and medium particles.

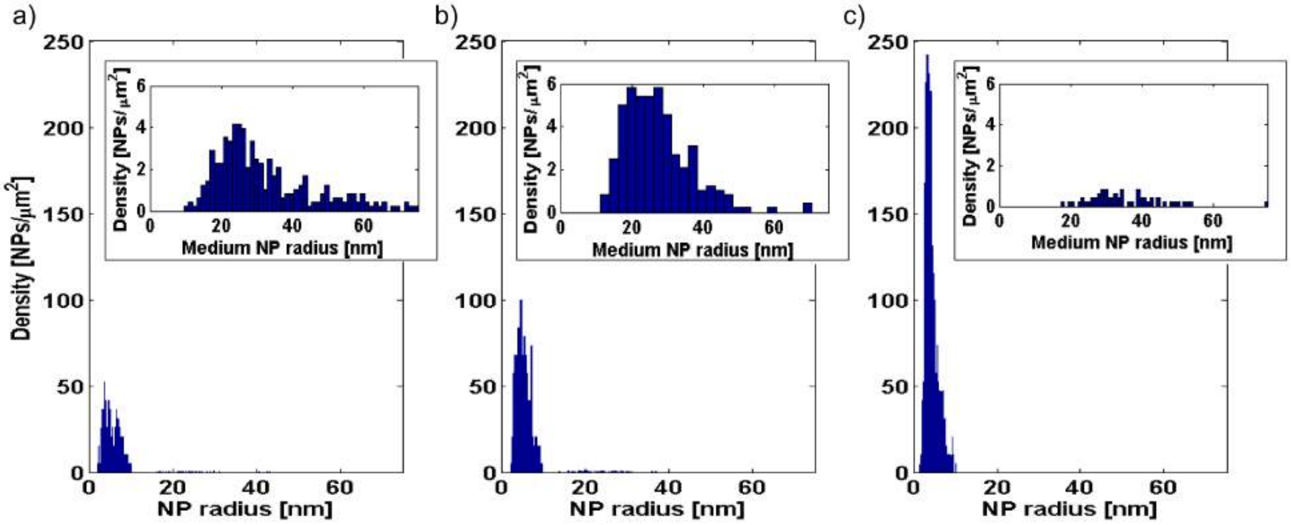


Figure S. 4: Histogram of the number of particles on the substrate relative to their radius over a surface area of 1 $\mu$m$^2$ for a fluence $\phi$ = 1.12 J/cm$^2$ and line spacing (a) $L_s$ = 5 $\mu$m, (b) $L_s$ = 10 $\mu$m, and (c) $L_s$ = 30 $\mu$m, at a marking speed $v$ = 11 mm/s. The inserts are magnifications of the medium particle distributions.

## Movie S. 1

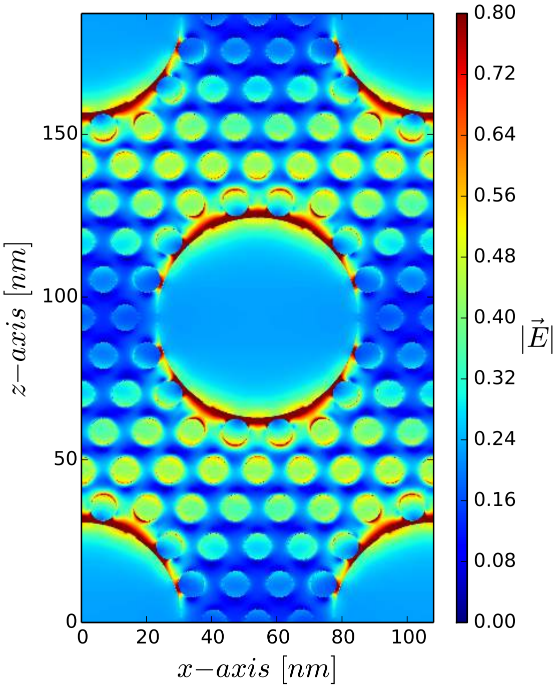


Figure S. 5: Frame extracted from Movie S. 1 showing the time evolution of the plane-wave pulse ($z$-polarized, $y$-propagating) interacting with the nanoparticles (half-embedded into the surface). The $xz$-plane is cut 2 nm above the silver substrate.

## Movie S. 2

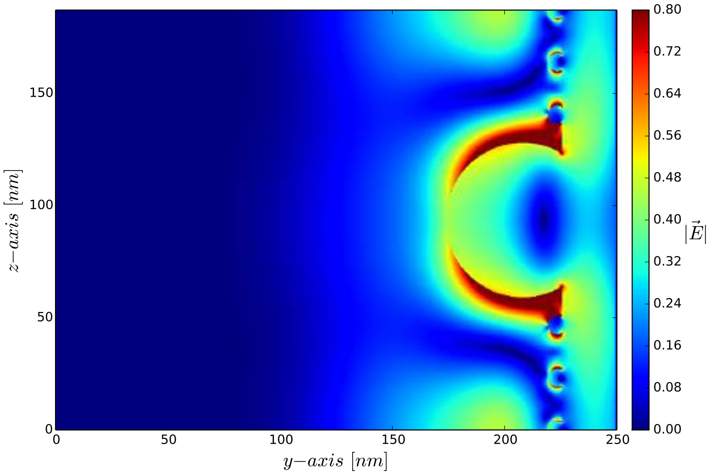


Figure S. 6: Frame extracted from Movie S. 2 showing time evolution of the plane-wave pulse ($z$-polarized, $y$-propagating) interacting with the nanoparticles (half-embedded into the surface). The $yz$ plane is cut through the middle of the medium size particle.

# References


[1] Wang, J. & Guo, C. Ultrafast dynamics of femtosecond laser-induced periodic surface pattern formation on metals. *Applied Physics Letters* **87**, 251914 (2005).

[2] Rechberger, W. *et al.* Optical properties of two interacting gold nanoparticles. *Optics Communications* **220**, 137–141 (2003).

[3] Romero, I., Aizpurua, J., Bryant, G. W. & García De Abajo, F. J. Plasmons in nearly touching metallic nanoparticles: singular response in the limit of touching dimers. *Optics Express* **14**, 9988–9999 (2006).

[4] Jain, P. K. & El-Sayed, M. A. Plasmonic coupling in noble metal nanostructures. *Chemical Physics Letters* **487**, 153–164 (2010).

[5] Liz-Marzán, L. M. Tailoring Surface Plasmons trough the Morphology and Assembly of Metal Nanoparticles. *Langmuir* **22**, 32–41 (2006).
